# Supplementary material for: Ab initio calculations of third-order elastic coefficients
Source: arXiv:2204.07608 source file (2022-11-13)
Supplement: Supplementary file 1 [file appendix.tex]

\section{Deformation and Lagrangian strain}

\subsection{Stress, strain and tensors under strain}
\label{sec:formalism:strain}

{\color{red} We found many additional work is because ref states are different...}
To build our formulation based on both continnum mechanics and solid-state physicists requires us to recognize their differences and try to layout a shared foundation that works for both fields.
Therefore, a clarification on reference state would come first in Subsec 2.1.1.
This clarification would allow us to address stress, SOEC and TOEC w.r.t. reference frames as foundation to our subsequent discussion. Sharing the traits of being strain derivatives of the energy density, Subsec 2.1.2 discribes how to change the reference state for these special tensors (i.e., how to move these tensors accross reference states). During the process, the different notations used by multiple classical papers referenced across the discussion might be confusing at times; under such occasions, our summary of the notations in Table~\ref{tab:history} might help facilitate the experience.

{\color{red}

There are tools in continuum mechanics...

There are already several classical papers by sesimologists and solid-state physicists in the field, but because .

}

\subsubsection{Reference frames}

In continnum mechanics, where theoretical tools are developed around a single strain connecting the unstrained and strained state, the two states can be reasonably referred to as ``initial'' and ``final''  \cite{dahlenTheoreticalGlobalSeismology1998};
in sesimology or mineral physics, where SOEC and aggregate moduli and accoustic velocities are being investigated vs. pressure, three states are usually relavent: (a) a natural state without external pressure (i.e., $P = 0$), (b) several intial states, usually under hydrostatic external pressure $P_i$, and (c) several present state by perturbing the initial state at presure $P_i$ with strain $\eta$ \cite{thurstonEffectiveElasticCoefficients1965}.
Fig.~\ref{fig:ref-states} (a) deplicts an example under this framework.
But these can get confusing in specific cases, e.g. (i) if we focus on $P=0$ only (e.g., Ref.~\cite{zhaoFirstprinciplesCalculationsSecond2007}), natural state and initial state are same; (ii) though we usually focus on initial and final states (e.g., Refs.~\cite{birchFiniteElasticStrain1947}), there are exceptions where ``natual'' states are used as the ``initial'' state strain-wise  (e.g., Ref.~\cite{thurstonEffectiveElasticCoefficients1965}); (iii) if we are calculating a pressure derivative of SOEC numerically, between initial states of $P_i$ and $P_j = P_i + \delta P$, we need to choose one as ``initial'' and one as ``final'' strain-wise.

{\color{red}
In this study, we try to be careful about them; reference state for the coordinates will be labeled with a superscript ``$\square^{(\square)}$'' if necessary.
The next subsection will cover a single strain only. But when tensors of two strains are involved, we will be chanigng reference frame for inital state.
}

\subsubsection{Deformation and strain}

Assume the coordinate gradient in ``initial'' (1) and ``current'' (1') state are $x_i^{(1)}$ and $x_i'^{(1')}$  ($i,i'=1,2,3$),  the deformation matrix, $F^{(1':1)}$ connecting the two states, its components $F_{i'i}^{(1':1)}$ are given by
\begin{equation}
F_{i'i}^{(1':1)} =  \frac{\partial x_{i'}^{(1')}}{\partial x_i^{(1)}} \quad .
\end{equation}
\textit{Ab initio} simulations focus on lattice parameters. Assume the $i$-th component of the $j$-th lattice vectors of the initial and current lattice vectors are $a^{(1)}_{ij}$ and $a^{(1')}_{i'j}$, because the deformation is uniform,  they are related by $F_{i'i}$ by $a^{(1')}_{i'j} = F^{(1':1)}_{i'i} a^{(1)}_{ij}$.

If we designate the initial state as state (1) and final state as state (1'), the Lagrangian strain ($\eta_{ij}$) can be obtained from deformation matrix $F$ by
\begin{equation}
\eta = \frac{1}{2}\big(F^\mathrm{T} F - 1\big) \quad .
\end{equation}
Obviously Lagrangian strain is symmetric, and does not contain the rotation information.
Therefore, $f: F \to \eta$ is one-to-one, but not inversely \cite{zhaoFirstprinciplesCalculationsSecond2007}.
%Assume unitary tranformation $U^\mathrm{T}U = I$, relating $F$ and $F'$ by $F' = U^\mathrm{T}FU$,
Because $\eta$ is symmetric, $(2\eta + I)$ is symmetric, it is diagonalizable as
\begin{equation}
F^\mathrm{T}F = (2\eta + I) = U^{-1} \Sigma U \quad .
\end{equation}
with $\Sigma$ being the eigenvector of $(2\eta + I)$. Therefore, a symmtric $F$ can be retrived from $\eta$ by
%The relavant deformation matrices ($F_{ij}$) can be obtained by
\begin{equation}
F = U^{-1} \Sigma^{1/2} U \quad .
\end{equation}
%The deformation matrices $F_{ij}$ obtained in this way is always symmetric.

Finally, we have Jacobian $J$, a scalar, denotes volume ($V$) or density ($\rho$) change
\begin{equation}
J^{(1':1)} = \frac{ V^{(1')} }{ V^{(1)} } = \frac{ \rho^{(1)} }{ \rho^{(1')} } \quad .
\end{equation}
It is can also be obtained from $F$ by
\begin{equation}
J = \det F ~ .
\end{equation}

\begin{figure}
\centering
\includegraphics[width=.45\textwidth]{figures/FIG1.png}
\caption{(a) Relationships between different states of reference: natual state, initial state, strained state and the Lagrangian strains connecting these states. (b, c) Formula for changing reference state for stress and SOEC tensors.}
\label{fig:ref-states}
\end{figure}

\subsubsection{Moving tensors across the reference frames}

Stress ($T_{ij}$), SOEC ($A_{ijkl}$), and TOEC ($A_{ijklmn}$) originate from the first, second-, and third-order derivatives of energy density w.r.t. Lagrangian strain,
\begin{align}
T_{ij} &= \rho \frac{\partial E}{\partial\eta_{ij}}, \\
A_{ijkl} &= \rho \frac{\partial^2 E}{\partial\eta_{ij} \partial\eta_{kl}}, \label{eq:def-soec}\\
A_{ijklmn} &= \rho \frac{\partial^3 E}{\partial\eta_{ij} \partial\eta_{kl} \partial\eta_{mn}}, \label{eq:def-toec}
\end{align}
where $\rho = 1/V$ is the density of the ``initial'' state, $E$ is the free-energy. Note here we use $A_{ijkl}$, $A_{ijklmn}$ to denote the derivatives to distinguish them from $C_{ijkl}$, $C_{ijklmn}$ the SOEC and TOEC that is measured and reported in geophysical research, which are different when $P \neq 0$ as will be further discussed in Secs.~\ref{sec:formalism:pressure-derivative} and \ref{sec:formalism:strain-induced}. 

\color{red}

In continnum mechanics, under a deformation $F_{i'i}$, 
Stress w.r.t. the current state is Cauchy-Lagrangian stress $T^\mathrm{L}$, and w.r.t. the (?) state second Piola-Kirchoff stress $T^\mathrm{SK}$, their transformation is given by
\begin{equation}
T^\mathrm{SK}_{i'j'} = J^{-1} F_{i'i} F_{j'j} T^\mathrm{L}_{ij}
\end{equation}
This could be more general,

We note that sometimes... these could get quite confusing ...

$\rho$ is transformed by $J^{-1}$, each $\eta_{ij}$ is transformed by $F_{i'i}^{-1} F_{j'j}^{-1}$

Therefore, the transformation rule for SOEC is

\begin{equation}
T_{i'j'} = J^{-1} F_{i'i} F_{j'j} T_{ij} ???
\end{equation}
\begin{equation}
A_{i'j'k'l'} = J^{-1} F_{i'i} F_{j'j} F_{k'k} F_{l'l} A_{ijkl} ???
\end{equation}
A rule of thumb is, the number of $F$ will match the number of subscript indices.

\normalcolor

\section{Connections with previous work}

\section{Finite strain fitting of SOEC and TOEC}

Eulerian strain with reference volume $V^\circ$ or reference lattice parameter $a^\circ$ is

\begin{equation}
f=\frac{1}{2}\left[\left(\frac{a^{\circ}}{a}\right)^{2}-1\right]=\frac{1}{2}\left[\left(\frac{V^{\circ}}{V}\right)^{\frac{2}{3}}-1\right]
\end{equation}

The 3rd-order finite strain EoS assumes

\begin{equation}
E(V)=\alpha_{3} f^{3}+\alpha_{2} f^{2}+\alpha_{1} f+\alpha_{0}
\end{equation}

Definition of pressure is $P=-\partial E/ \partial V$, therefore we have

\begin{equation}
P=-\frac{\partial E}{\partial V}=-\frac{\partial E}{\partial f} \frac{\partial f}{\partial V}=-\left(3 \alpha_{3} f^{2}+2 \alpha_{2} f+\alpha_{1}\right)\left(\frac{\partial f}{\partial V}\right)
\end{equation}

Because $\partial f / \partial V=\frac{1}{3}(2 f+1) V^{-1}$, $PV$ is a third-order polynomial of $f$, assume
\color{red}

\begin{equation}
P V=\beta_{3} f^{3}+\beta_{2} f^{2}+\beta_{1} f+\beta_{0}
\end{equation}

Then we have the bulk moduli $\kappa$, or thermodynamic SOEC $A_{ijkl}$, given by

\begin{equation}
\kappa=V \frac{\partial P}{\partial V}=V \frac{\partial P}{\partial f} \frac{\partial f}{\partial V}=\left(3 \beta_{3} f^{2}+2 \beta_{2} f+\beta_{1}\right) \cdot \frac{1}{3}(2 f+1)
\end{equation}

Also a third order polynomial of $f$. Higher order strain derivative of $\kappa$, e.g. TOEC, is similarly a third-order polynomial of $f$.

The constraint $P(V_0)=0$ gives a special reference volume $V^\circ=V_0$ that effectively eliminates $\alpha_1$, results in the more commonly known 3rd order Birch-Murnaghan equation of states. The use of $V_0$ instead of an arbitrary $V^\circ$ does not change the form or order of these polynomial equation (C.2)-(C.5) in general.

\normalcolor
